# Supplementary material for: The Role of Compositionality in Constructing Complementarity Classical Structures Within Qubit Systems
Source: arXiv:2105.11966 source file (2021-05-24)
Supplement: Supplementary file 1 [file appendix.tex]

\subsection{$cw_{2,3}$}
\input{list/CD1}

\subsection{$cw_{2,4}$}
\input{list/CD2}

\newpage
\subsection{$cw_{3,1}$}
\input{list/CD3}

\subsection{$cw_{3,2}$}
\input{list/CD4}

\subsection{$cw_{3,3}$}
\input{list/CD5}

\subsection{$cw_{3,4}$}
\input{list/CD6}

\subsection{$cw_{3,5}$}
\input{list/CD7}

\subsection{$cw_{3,6}$}
\input{list/CD8}

\subsection{$cw_{4,1}$}
\input{list/CD9}

\subsection{$cw_{4,2}$}
\input{list/CD10}

\subsection{$cw_{4,3}$}
\input{list/CD11}

\subsection{$cw_{4,4}$}
\input{list/CD12}

\subsection{$cw_{4,5}$}
\input{list/CD13}

\subsection{$cw_{4,6}$}
\input{list/CD14}

\newpage
\subsection{$cw_{4,7}$}
\input{list/CD15}

\subsection{$cw_{4,8}$}
\input{list/CD16}

\subsection{$cw_{4,9}$}
\input{list/CD17}

\subsection{$cw_{4,10}$}
\input{list/CD18}

\subsection{$cw_{4,11}$}
\input{list/CD19}

\subsection{$cw_{5,1}$}
\input{list/CD20}

\newpage
\subsection{$cw_{5,2}$}
\input{list/CD21}

\subsection{$cw_{5,3}$}
\input{list/CD22}

\subsection{$cw_{5,4}$}
\input{list/CD23}

\subsection{$cw_{6,1}$}
\input{list/CD24}

\newpage
\subsection{$cw_{6,2}$}
\input{list/CD25}
